# Supplementary material for: Efficient Diffusion Models: A Comprehensive Survey from Principles to Practices
Source: arXiv:2410.11795 source file (2024-10-16)
Supplement: Supplementary file 1 [file 9_appendix.tex]

\section{Symbol Table}

\begin{table}[ht]
\centering
\caption{Symbol Table.}
\begin{tabular}{l|c}
\toprule
\textbf{Symbol} & \textbf{Meaning} \\ 
\midrule
$x$ & \\
$y$ &  \\
$h$ &  \\
$L$ &  \\

\bottomrule
\end{tabular}
\label{tab:stat}
\end{table}
